# Supplementary material for: Is my Meeting Summary Good? Estimating Quality with a Multi-LLM Evaluator
Source: arXiv:2411.18444 source file (2024-11-27)
Supplement: Supplementary file 1 [file A_Appendix_Bias.tex]

\label{sec:appendix_bias}

We report the performance as average Likert scores on the eight error types for summaries generated by LED \cite{BeltagyPC20}, DialogLED \cite{ZhongLXZ22}, Pegasus-X \cite{PhangZL22}, GPT-3.5, and Phi-3 for an evaluation architecture using MADP with and without instances from multiple model families in \Cref{tab:bias}.
The multiple model families consist of GPT4, Phi-3-medium-128k \cite{AbdinJAA24}, Llama 3.2 11b \cite{MetaAI24}, and Gemini 1.5 Flash \cite{GeminiTeamRST24}.
GPT4 takes here the role of the moderator and is refined by the other models.

We observe no notable difference depending on the summarizing model or error type.
We conclude, that we have a minimal risk of bias and hence can rely on a single model for \metric{}.

\begin{table*}[ht]
    \centering
    \small
    \begin{tabular}{lccccccccc}
        \toprule
        \textbf{Sum model} & Eval Setup & \textbf{OM} & \textbf{REP} & \textbf{INC} & \textbf{COR} & \textbf{HAL} & \textbf{LAN} & \textbf{STR} & \textbf{IRR} \\
        \midrule
        \multirow{2}{*}{LED}  & GPT4 &  4.08 & 3.74 & 4.03 & 3.39 & 3.81 & 3.76 & 3.83 & 3.38 \\
                              & Multi &  4.30 & 3.93 & 4.05 & 3.96 & 3.94 & 3.80 & 4.03 & 3.74 \\
        \multirow{2}{*}{DialogLED}  & GPT4 &  4.30 & 3.93 & 4.05 & 3.96 & 3.94 & 3.80 & 4.03 & 3.74 \\
                              & Multi &  4.30 & 3.93 & 4.05 & 3.96 & 3.94 & 3.80 & 4.03 & 3.74 \\
        \multirow{2}{*}{PegasusX}  & GPT4 &  4.30 & 3.93 & 4.05 & 3.96 & 3.94 & 3.80 & 4.03 & 3.74 \\
                              & Multi &  4.30 & 3.93 & 4.05 & 3.96 & 3.94 & 3.80 & 4.03 & 3.74 \\
        \multirow{2}{*}{GPT-3.5} & GPT4 &  4.08 & 3.74 & 4.03 & 3.39 & 3.81 & 3.76 & 3.83 & 3.38 \\
                                 & Multi &  4.08 & 3.74 & 4.03 & 3.39 & 3.81 & 3.76 & 3.83 & 3.38 \\
        \multirow{2}{*}{Phi-3}   & GPT4 &  4.08 & 3.74 & 4.03 & 3.39 & 3.81 & 3.76 & 3.83 & 3.38 \\
                                 & Multi &  4.08 & 3.74 & 4.03 & 3.39 & 3.81 & 3.76 & 3.83 & 3.38 \\
        \bottomrule
    \end{tabular}
    \caption{Average Likert scores of our three-step approach using MADP with a single model (GPT4) and multiple models (Multi) involved in the discussion. The scores are split according to the language model used to generate the summary that is being evaluated.}
    \label{tab:bias}
\end{table*}
